# Supplementary material for: Breathing Mode of a BEC Repulsively Interacting with a Fermionic Reservoir
Source: arXiv:1812.06445 ancillary file (2018-12-16)
Supplement: Supplementary file 1 [file Supplemental_breathing.pdf]

# Supplemental Material: Breathing Mode of a BEC Repulsively Interacting with a Fermionic Reservoir

Bo Huang (黄博),<sup>1,\*</sup> Isabella Fritsche,<sup>1,2,†</sup> Rianne S. Lous,<sup>1,2</sup> Cosetta Baroni,<sup>1,2</sup>

Jook T. M. Walraven,<sup>1,3</sup> Emil Kirilov,<sup>1,4</sup> and Rudolf Grimm<sup>1,4</sup>

<sup>1</sup>*Institut für Quantenoptik und Quanteninformation (IQOQI),*

*Österreichische Akademie der Wissenschaften, 6020 Innsbruck, Austria*

<sup>2</sup>*Institut für Experimentalphysik und Zentrum für Quantenphysik, Universität Innsbruck, 6020 Innsbruck, Austria*

<sup>3</sup>*Van der Waals-Zeeman Institute, Institute of Physics, University of Amsterdam, Science Park 904, 1098 XH Amsterdam, The Netherlands*

<sup>4</sup>*Institut für Experimentalphysik, Universität Innsbruck, 6020 Innsbruck, Austria*

(Dated: December 16, 2018)

## ANALYSIS OF THE OSCILLATION DATA

Here, we explain the fitting procedure for our data by which we extract the results presented in the main text. We obtain the data by taking absorption pictures of the partial BECs. We fit the images with a bimodal distribution (assuming a simple Thomas-Fermi distribution for the BEC) and extract the width of the condensed part of the atomic cloud in both the radial and the axial ( $z$ ) direction. By varying the time after the excitation (see Fig. 2 in the main text), we typically record six oscillation periods of the radial width. In Fig. S1(a) we show an extended time evolution of the radial width  $R$ , which shows the dynamics on a longer time scale. We observe an oscillation at a frequency  $\omega$ , which corresponds to the radial breathing mode of the BEC. Its frequency is twice the trap frequency of the bosons. In addition to that, we notice a slow background oscillation. This corresponds to an axial mode, which is known as the quadrupole mode for BECs in elongated traps [1]. The excitation of this mode is visible in the time evolution of the axial width  $R_z$  depicted in Fig. S1(b). It takes place on a much longer time scale than the radial breathing mode, because of the large aspect ratio (7.6) in our elongated trap.

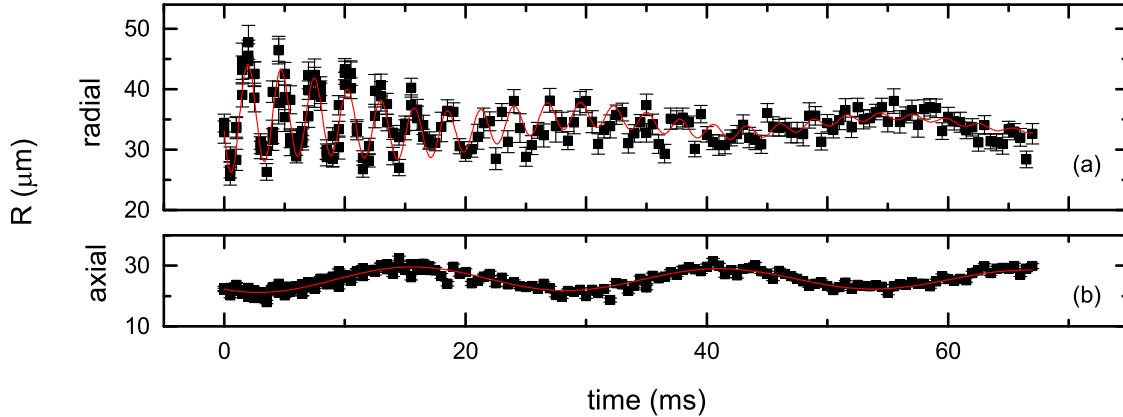

FIG. S1. Long-term time evolution of the BEC size  $R$  in the radial and the axial directions at  $a_{bf} = 362a_0$  ( $a_c/a_{bf} \approx 1.66$ ) and  $N_b/N_f = 0.18$ . The error bars show the  $1\sigma$  error of the bimodal fit. Panel (a) shows the fast radial mode on the background of a slow oscillation induced by the axial mode and panel (b) the slow axial mode. The results of the fits are presented as solid red curves.

We obtain the radial breathing mode frequency, by fitting  $R(t)$  by a damped harmonic oscillation with a slowly oscillating background,

$$R(t) = R_0 + Ae^{-\gamma t} \sin(\omega t - \phi) + A_z e^{-\gamma_z t} \sin(\omega_z t - \phi_z), \quad (\text{S1})$$

where the free parameters of interest are the frequency  $\omega$  and the damping rate  $\gamma$ . Other free parameters of this fitting function are the offset  $R_0$ , the amplitudes  $A$  and  $A_z$  and the phases  $\phi$  and  $\phi_z$ . We determine the axial frequency

$\omega_z$  and damping rate  $\gamma_z$  independently by fitting a damped sinusoidal function to the time evolution of the axial width  $R_z$ , as depicted in Fig. S1(b). For most of the data presented in the main text we record about six breathing mode periods. This means that each set of oscillations only shows a part of a period of the axial mode. Therefore the obtained values of  $\omega$  and  $\gamma$  are largely insensitive to the exact values of the axial parameters  $\omega_z$  and  $\gamma_z$ . For this reason we take only one data set for the axial mode and then fix  $\omega_z$  and  $\gamma_z$  in Eq. (S1) for the analysis of all measurements of the radial breathing mode.

## THEORETICAL MODELS

Here we briefly summarize the two models, the adiabatic Fermi sea (AFS) and full phase-separation (FPS), which we used in the main text to describe our experimental observations. Both models approximate the elongated mixture as a cylindrical system, where the density distribution in radial direction over the whole z-axis (axial direction) corresponds to the radial density at the center of the original system. Detailed studies on these models as well as another numerical model applying the test-particle method [2] for fermions will be discussed separately [3].

### Adiabatic Fermi sea (AFS) model

For each given set of parameters, e.g.  $\{a_{bf}, N_b, N_f\}$ , we obtain the equilibrium state of the Bose-Fermi mixture via a numerical procedure as described in Ref. [4]. Then we approximate our elongated mixture with a cylindrical system, of which the radial density profiles take the numerical values in the plane at the trap center ( $z = 0$ ). Particularly, the order parameter of the BEC at equilibrium is given by the BEC density as  $\psi_0 = \sqrt{n_{b0}}$ . In order to simulate the oscillations, we start with a perturbed order parameter  $\psi = \psi_0 + \delta\psi$ , e.g. the  $\psi_0$  for a slightly different  $a_{bf}$ . Then we let  $\psi$  evolve in time following

$$i\hbar \frac{\partial \psi}{\partial t} = -\frac{\hbar^2}{2m_b} \nabla^2 \psi + g_{bb} \psi^* \psi^2 + (U_b + g_{bf} n_f) \psi, \quad (\text{S2})$$

where  $g_{bb} = 4\pi\hbar^2 a_{bb}/m_b$  and  $g_{bf} = 2\pi\hbar^2 a_{bf}(m_b + m_f)/m_b m_f$  are coupling constants, and  $U_b$  is the external trapping potential for bosons. The fermion density is

$$n_f = C(\mu_f - U_f - g_{bf} n_b)^{3/2} H(\mu_f - U_f - g_{bf} n_b), \quad (\text{S3})$$

where  $C = (2m_f/\hbar^2)^{3/2}/2\pi^2$ ,  $\mu_f$  is the global chemical potential of fermions,  $U_f$  the trapping potential for fermions,  $n_b = \psi^* \psi$  the BEC density, and  $H$  the Heaviside step function. Furthermore we apply the fermionic reservoir approximation [4], which assumes a constant global chemical potential  $\mu_f$ .

The weighted averaged width of the cylindrical BEC,  $R = \int r^2 n_b(r) dr / \int r n_b(r) dr$ , is recorded as a function of time up to the typical duration of observations and fitted with a cosine function to extract the oscillation frequency  $\omega$  for the current set of parameters.

### Full phase separation (FPS) model

At the limit of large  $a_{bf}$  when the full phase separation occurs, we first study the dynamics of the two components separately within the Thomas-Fermi approximation. Then the frequency of the collective mode is determined by matching the boundary conditions, i.e. velocity and pressure, at the interface. Following a procedure introduced in Ref. [5] for a spherical case, we investigate the oscillation for a cylindrical mixture, which is more relevant to our experiment. We note that the currently ignored finite kinetic energy of the BEC at the interface can be included as a surface tension effect [6]. However, to adhere to a simple and transparent picture here, we neglect the contribution off the surface tension term, which involves several further assumptions and tends to give a slightly higher frequency shift.

In the cylindrical case, the perturbation of the BEC density is described by

$$\delta n_b(r) \propto F \left( \frac{1 + \sqrt{1 + 2\omega^2/\omega_b^2}}{2}, \frac{1 - \sqrt{1 + 2\omega^2/\omega_b^2}}{2}, 1, \frac{r^2}{R^2} \right), \quad (\text{S4})$$

where  $F$  is the hypergeometric function  ${}_2F_1$ ,  $\omega$  the frequency of the collective mode,  $\omega_b$  the trapping frequency of bosons, and  $R$  the Thomas-Fermi radius of the BEC. For a phase-separated mixture in a harmonic trap, the value of  $R$  is determined by the chemical potential  $\mu_b$  of the compressed BEC via  $\mu_b = m_b \omega_b^2 R^2 / 2$ .

The ansatz describing the deformation of the Fermi surface in a cylindrical system is  $f = f_0 + \delta(|\mathbf{p}| - p_f) u(r, \alpha, \beta) e^{-i\omega t}$ , where  $\alpha = \cos \phi$  as  $\phi$  is the angle between the momentum  $\mathbf{p}$  and the position  $\mathbf{r}$  in the radial plane,  $\beta = \cos \theta$  as  $\theta$  is the angle between  $\mathbf{p}$  and the  $z$ -axis (axial direction), and  $p_f(r) = \sqrt{2m_f[\mu_f - U_f(r)]}$  is the local Fermi momentum. Then the fermion perturbation has a solution as

$$u(r, \alpha, \beta) = \mathcal{F}_1[L^2] \mathcal{F}_2[v_z^2] e^{-i\omega\tau/2} \quad (\text{S5})$$

where

$$L^2 = \omega_f^2 r^2 (R_f^2 - r^2) (1 - \alpha^2) (1 - \beta^2), \quad (\text{S6})$$

$$v_z^2 = \omega_f^2 (R_f^2 - r^2) \beta^2, \quad (\text{S7})$$

$\mathcal{F}_1[x]$  and  $\mathcal{F}_2[x]$  are arbitrary differentiable functions of  $x$ , the angular momentum  $L$  and velocity  $v_z$  in the axial ( $z$ ) direction are constants of motion.  $R_f$  is the Thomas-Fermi radius. The single fermion trajectory period  $\tau$  is

$$\tau(r, \alpha, \beta) = \frac{\psi_0 - \arctan[2\alpha/g(r, \beta)]}{\omega_f}, \quad (\text{S8})$$

where  $\psi_0 = \pi H[g(r, \beta)]$ ,  $g(r, \beta) = \sqrt{(1 - \beta^2)(R_f^2 - r^2)}/r - r/\sqrt{(1 - \beta^2)(R_f^2 - r^2)}$  and the domain of  $\alpha$  and  $\beta$  is  $[0, 1]$ . For other values of  $\alpha$  and  $\beta$ , we have  $\tau(r, -\alpha, \beta) = -\tau(r, \alpha, \beta)$  and  $\tau(r, \alpha, -\beta) = \tau(r, \alpha, \beta)$ . In an intuitive picture, fermions repeatedly bounce off ( $\alpha > 0$ ) the Bose-Fermi interface and fall back (with  $\alpha' = -\alpha$ ) to it, because of the trapping potential, at a time interval of  $\tau$ .

We obtain the collective motion frequency  $\omega$  by matching the boundary conditions at the interface  $r = \zeta$ . In the first place, the pressures of the BEC and the fermions should be equal when the surface tension is ignored [6]. The pressure of the excited Fermi sea is given by the momentum flux  $\Pi(r) = (1/m_f h^3) \int d^3\mathbf{p} \alpha^2 (1 - \beta^2) p^2 f(\mathbf{p}, r)$  in the radial direction. Moreover, assuming a perfect phase-separation without exchange of particles, the radial speeds of the two components are equal at the interface. We now arrive at the equation for  $\omega$  as

$$\frac{\partial_r F}{F} = \frac{\omega^2 m_b n_b}{\frac{p_f^4 C_\Pi}{(2\pi\hbar)^3} - \partial_r (P_b - P_f)}, \quad (\text{S9})$$

where  $C_\Pi = 8\omega \int_0^{\pi/2} d\phi \int_0^1 d\beta (1 - \beta^2)^{3/2} \cos^3 \phi \cot(\omega\tau/2)$ . Finally we apply the parameters at the interface into Eq. (S9) and solve it to get  $\omega$ .

## ROLE OF THE ATOM NUMBER RATIO

Here we clarify the dependence of  $\omega$  in the full phase-separation regime on the atom number ratio  $N_f/N_b$ , as this dependence is shown in Fig. 4 of the main text. In view of our theoretical models, the dependence can be understood by considering the FPS model and apply further approximations to Eq. (S9). First we ignore the fluctuation of the Fermi momentum flux, i.e. the term with  $C_\Pi$ , and arrive at an AFS model in the Thomas-Fermi limit. Secondly, we assume  $\zeta \ll R_f$  and drop  $\partial_r P_f$ . Finally, we consider the limit of  $N_f/N_b \gg 1$ , where the BEC is tightly squeezed ( $\zeta \ll R$ ) and  $n_b$  becomes a constant. In this condition, Eq. (S9) reduces to  $\omega^2/\omega_b^2 = (r\partial F/\partial r)/F$ , the pressure balance condition requires  $R^4 \propto R_f^5$ , and the atom number conservation corresponds to  $N_b \propto R^2 \zeta^3$  and  $N_f \propto R_f^6$ . By solving the simplified equation, we find  $\omega/\omega_b \propto (N_b/N_f^{25/24})^{1/3} \sim (N_b/N_f)^{1/3}$ . Consequently, it is valid to approximate  $\omega/\omega_b$  (and  $\omega/\omega_0$  in the main text) as a function of  $N_b/N_f$ .

In the numerical calculations, we use a total atom number of  $1.0 \times 10^5$  and change the atom number ratio  $N_f/N_b$  to study the corresponding variation of  $\omega$ . To justify that any change of the total atom number has only minor influences on our results, we test the dependence of  $\omega$  on the total atom number. We verify that if we increase the total atom number by a factor of two while keeping  $N_f/N_b$  constant, the breathing mode frequency increases by less than 1% (4%) in the FPS (AFS) model.

In the experiment we change the atom number ratio by varying the duration of loading atoms into the magneto-optical trap. In our system we consecutively load Li and K. While loading the latter, the Li atom number decays. Therefore to increase the atom number ratio  $N_b/N_f$  we increase the K loading time, which increases  $N_b$  and reduces  $N_f$ . We tune  $N_b$  from  $6.6 \times 10^3$  to  $2.3 \times 10^4$  while the corresponding  $N_f$  is between  $2.2 \times 10^5$  and  $1.0 \times 10^5$ .

## OTHER MODES AND THE ATTRACTIVE SIDE OF THE FESHBACH RESONANCE

We briefly report some further observations in our system. First we look into the radial breathing mode frequency at negative  $a_{bf}$  values. Our measurements on the attractive side of the Feshbach resonance are limited to  $|a_{bf}| \lesssim 600$ . For very strong attractive interactions the oscillations are not well-defined, because the mixture is close to the regime where the BEC undergoes collapse [7, 8] and rapidly decays. In this complex regime we see a small upshift in frequency, which reaches a maximum value of 6(2)%.

Secondly, we measure the frequency of the radial dipole mode at positive scattering lengths. We excite this oscillation by shortly switching on an additional trapping beam, which is slightly displaced and parallel to the beam that provides the radial confinement in the crossed optical dipole trap. This displaces the center of mass of the cloud. By switching off this excitation beam we release the sample into the original trap and record the oscillation. Our observations show that there is no interaction-induced shift on the level of 0.5%.

It would be interesting to study also frequency shifts in the low-lying axial modes, i.e. the axial dipole and the quadrupole mode. Due to their surface character these shifts are expected to be small. For the slow axial mode that we clearly observe in both panels in Fig. S1, the oscillations are of opposite phase. This points to the fact that the mode, as expected [1], is mainly a quadrupole mode and thus has predominant surface character. However, two reasons hinder the observation of the frequency shifts in our system. As mentioned before, the timescale of the axial modes is much longer than that of the radial modes. Consequently in the interesting regime, where the interaction is strong and frequency shifts may occur, the fast decay of the atom number leads to large errors in the frequency measurements and prevents us from resolving a frequency shift there. A large uncertainty in these measurements results from the excitation scheme in our experiment. In the time evolution of the axial dipole mode, for example, we observe various hints for higher-order excitations. For these reasons we can only state within an uncertainty of 8% that we do not see a frequency shift for these modes.

---

\* [Bo.Huang@uibk.ac.at](mailto:Bo.Huang@uibk.ac.at)

† I.F. and B.H. contributed equally to this work.

- [1] M.-O. Mewes, M. R. Andrews, N. J. van Druten, D. M. Kurn, D. S. Durfee, C. G. Townsend, and W. Ketterle, *Phys. Rev. Lett.* **77**, 988 (1996).
- [2] M. Brack and R. K. Bhaduri, *Semiclassical Physics* (Addison-Wesley Publishing Company, Inc., 1997).
- [3] B. Huang *et al.* (to be published).
- [4] R. S. Lous, I. Fritsche, M. Jag, F. Lehmann, E. Kirilov, B. Huang, and R. Grimm, *Phys. Rev. Lett.* **120**, 243403 (2018).
- [5] B. Van Schaeybroeck and A. Lazarides, *Phys. Rev. A* **79**, 033618 (2009).
- [6] B. Van Schaeybroeck, *Phys. Rev. A* **78**, 023624 (2008).
- [7] C. Ospelkaus, S. Ospelkaus, K. Sengstock, and K. Bongs, *Phys. Rev. Lett.* **96**, 020401 (2006).
- [8] M. Zaccanti, C. D'Errico, F. Ferlaino, G. Roati, M. Inguscio, and G. Modugno, *Phys. Rev. A* **74**, 041605 (2006).
